# Supplementary material for: PICABench: How Far Are We from Physically Realistic Image Editing?
Source: arXiv:2510.17681 source file (2026-01-04)
Supplement: Supplementary file 1 [file fig_State__Local_local_Explicit.tex]

\begin{figure}[t]
\begin{minipage}[t]{\linewidth}
\textbf{Intermediate Prompt:} Apply a local phase change to the red liquid in the martini glass so it becomes solid ice while respecting ... \\
\vspace{-0.5em}
\end{minipage}
\begin{minipage}[t]{\linewidth}
\centering
\newsavebox{\tmpboxakIntermediate}
\newlength{\minipageheightakIntermediate}
\sbox{\tmpboxakIntermediate}{
\begin{minipage}[t]{0.19\linewidth}
\centering
\includegraphics[width=\linewidth]{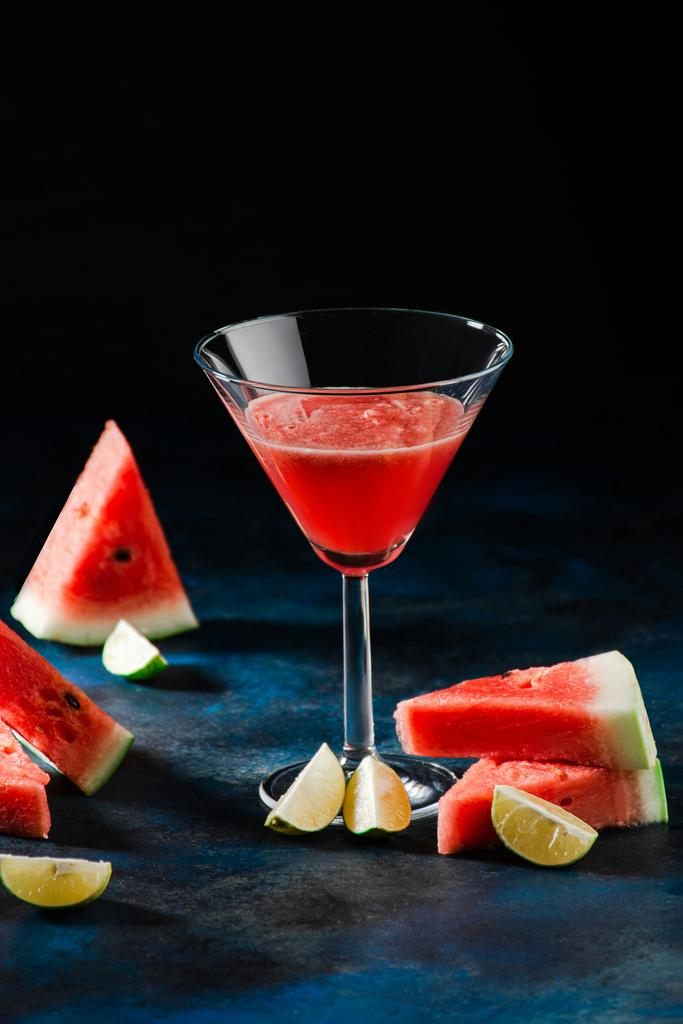}
\vspace{-1em}\textbf{\footnotesize Input}
\end{minipage}
}
\setlength{\minipageheightakIntermediate}{\ht\tmpboxakIntermediate}
\begin{minipage}[t]{0.19\linewidth}
\centering
\adjustbox{width=\linewidth,height=\minipageheightakIntermediate,keepaspectratio}{\includegraphics{iclr2026/figs/final_selection/State__Local__intermediate_0416_ahmadreza-rezaie-bPCU2srEeq4-unsplash_State_Local_frozen/input.png}}
\end{minipage}
\hfill
\begin{minipage}[t]{0.19\linewidth}
\centering
\adjustbox{width=\linewidth,height=\minipageheightakIntermediate,keepaspectratio}{\includegraphics{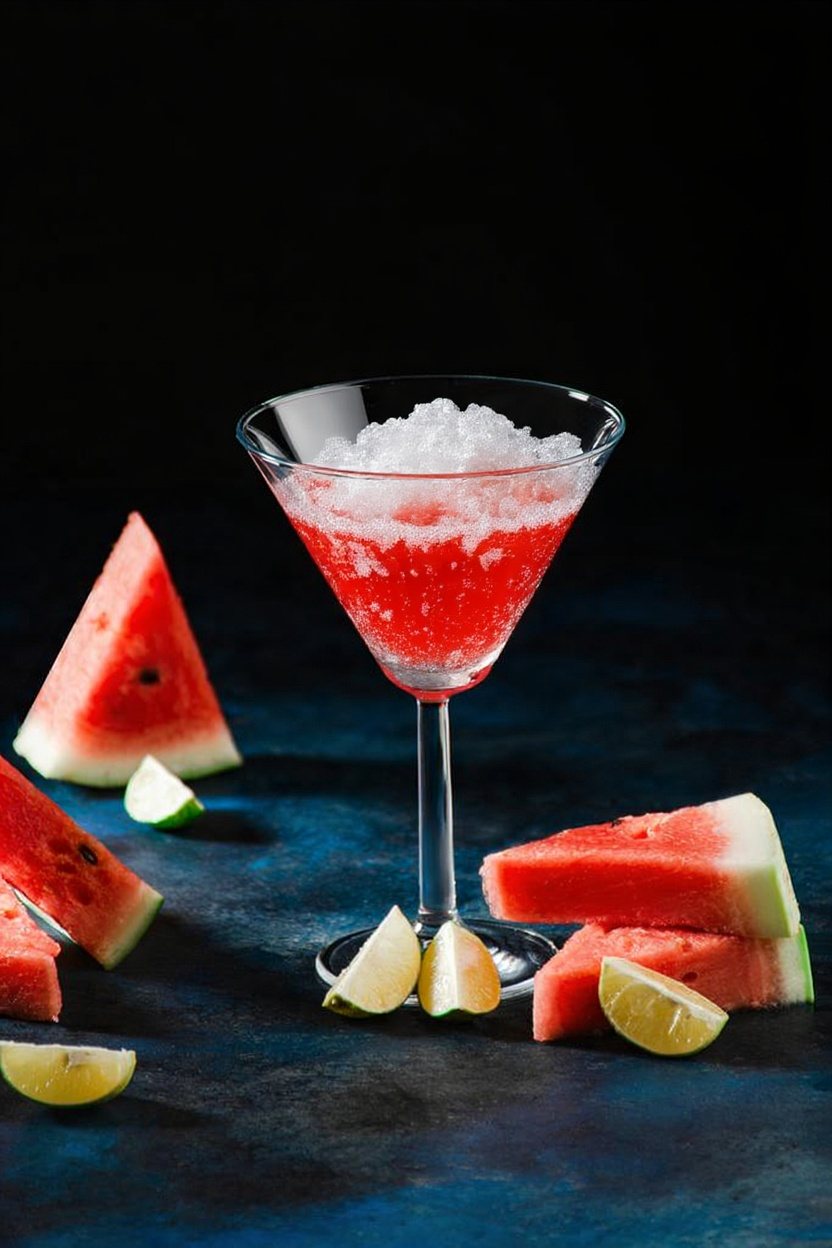}}
\end{minipage}
\hfill
\begin{minipage}[t]{0.19\linewidth}
\centering
\adjustbox{width=\linewidth,height=\minipageheightakIntermediate,keepaspectratio}{\includegraphics{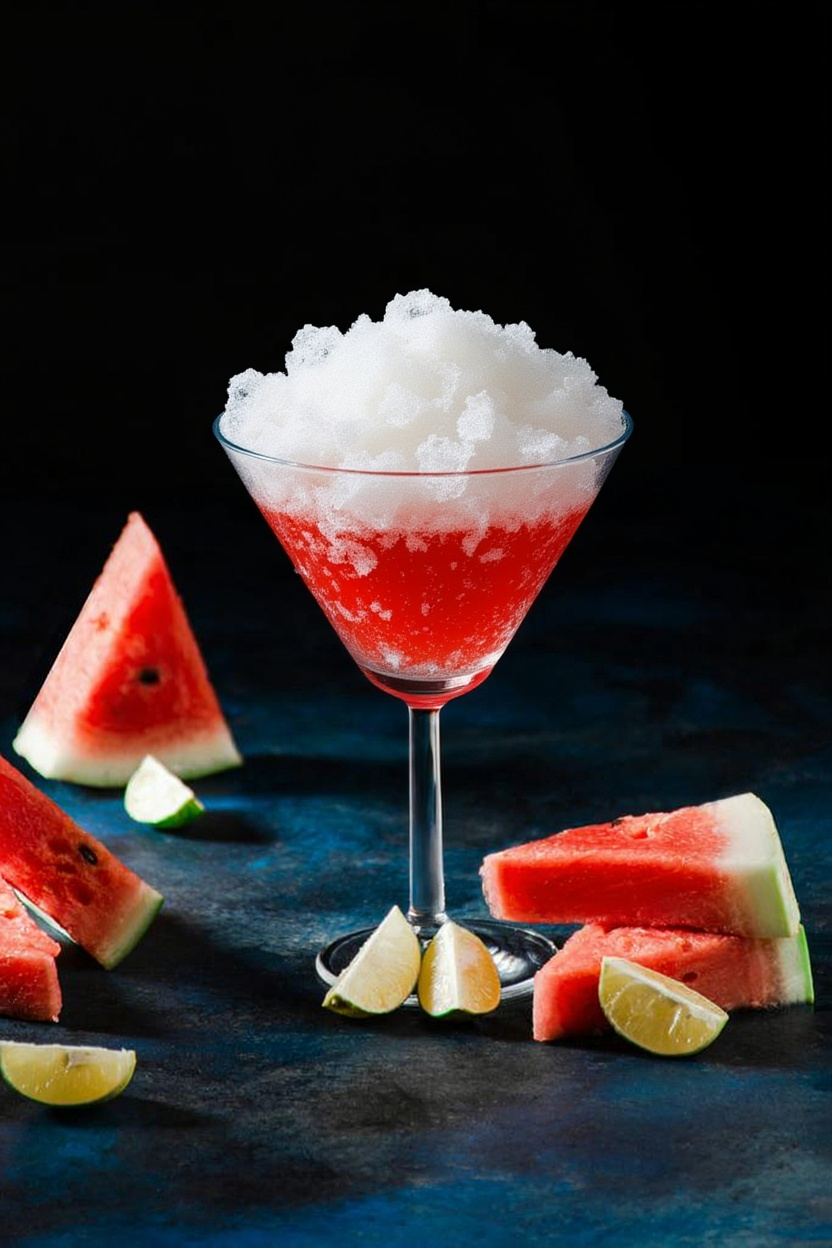}}
\end{minipage}
\hfill
\begin{minipage}[t]{0.19\linewidth}
\centering
\adjustbox{width=\linewidth,height=\minipageheightakIntermediate,keepaspectratio}{\includegraphics{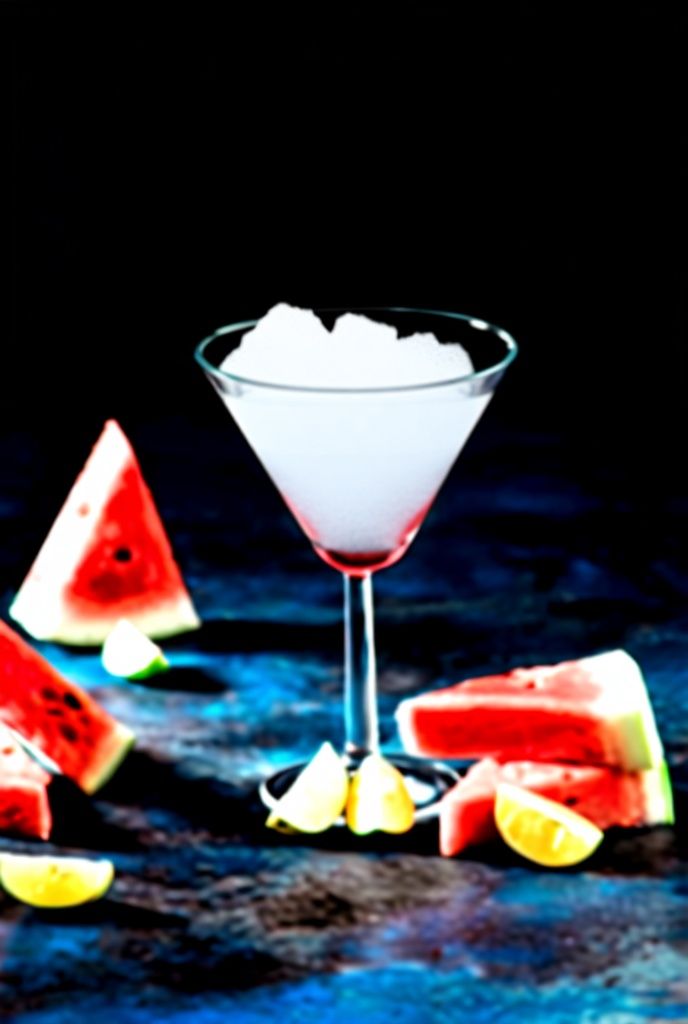}}
\end{minipage}
\hfill
\begin{minipage}[t]{0.19\linewidth}
\centering
\adjustbox{width=\linewidth,height=\minipageheightakIntermediate,keepaspectratio}{\includegraphics{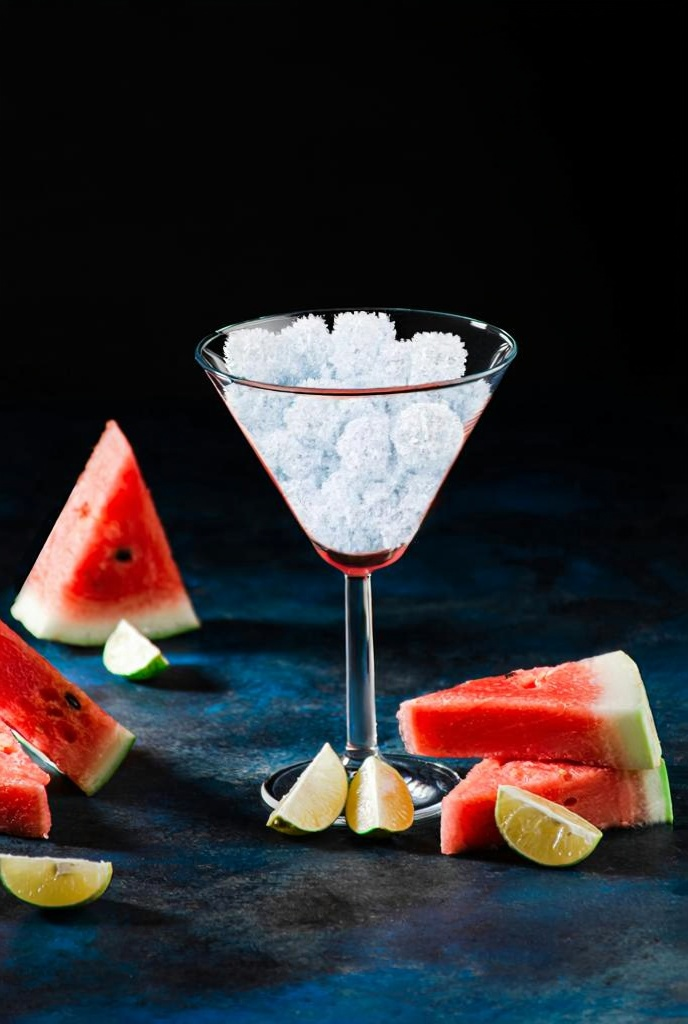}}
\end{minipage}\\
\begin{minipage}[t]{0.19\linewidth}
\centering
\vspace{-0.7em}\textbf{\footnotesize Input}    
\end{minipage}
\hfill
\begin{minipage}[t]{0.19\linewidth}
\centering
\vspace{-0.7em}\textbf{\footnotesize Ours}    
\end{minipage}
\hfill
\begin{minipage}[t]{0.19\linewidth}
\centering
\vspace{-0.7em}\textbf{\footnotesize Flux.1 Kontext}    
\end{minipage}
\hfill
\begin{minipage}[t]{0.19\linewidth}
\centering
\vspace{-0.7em}\textbf{\footnotesize BAGEL}    
\end{minipage}
\hfill
\begin{minipage}[t]{0.19\linewidth}
\centering
\vspace{-0.7em}\textbf{\footnotesize BAGEL-Think}    
\end{minipage}\\
\begin{minipage}[t]{0.19\linewidth}
\centering
\adjustbox{width=\linewidth,height=\minipageheightakIntermediate,keepaspectratio}{\includegraphics{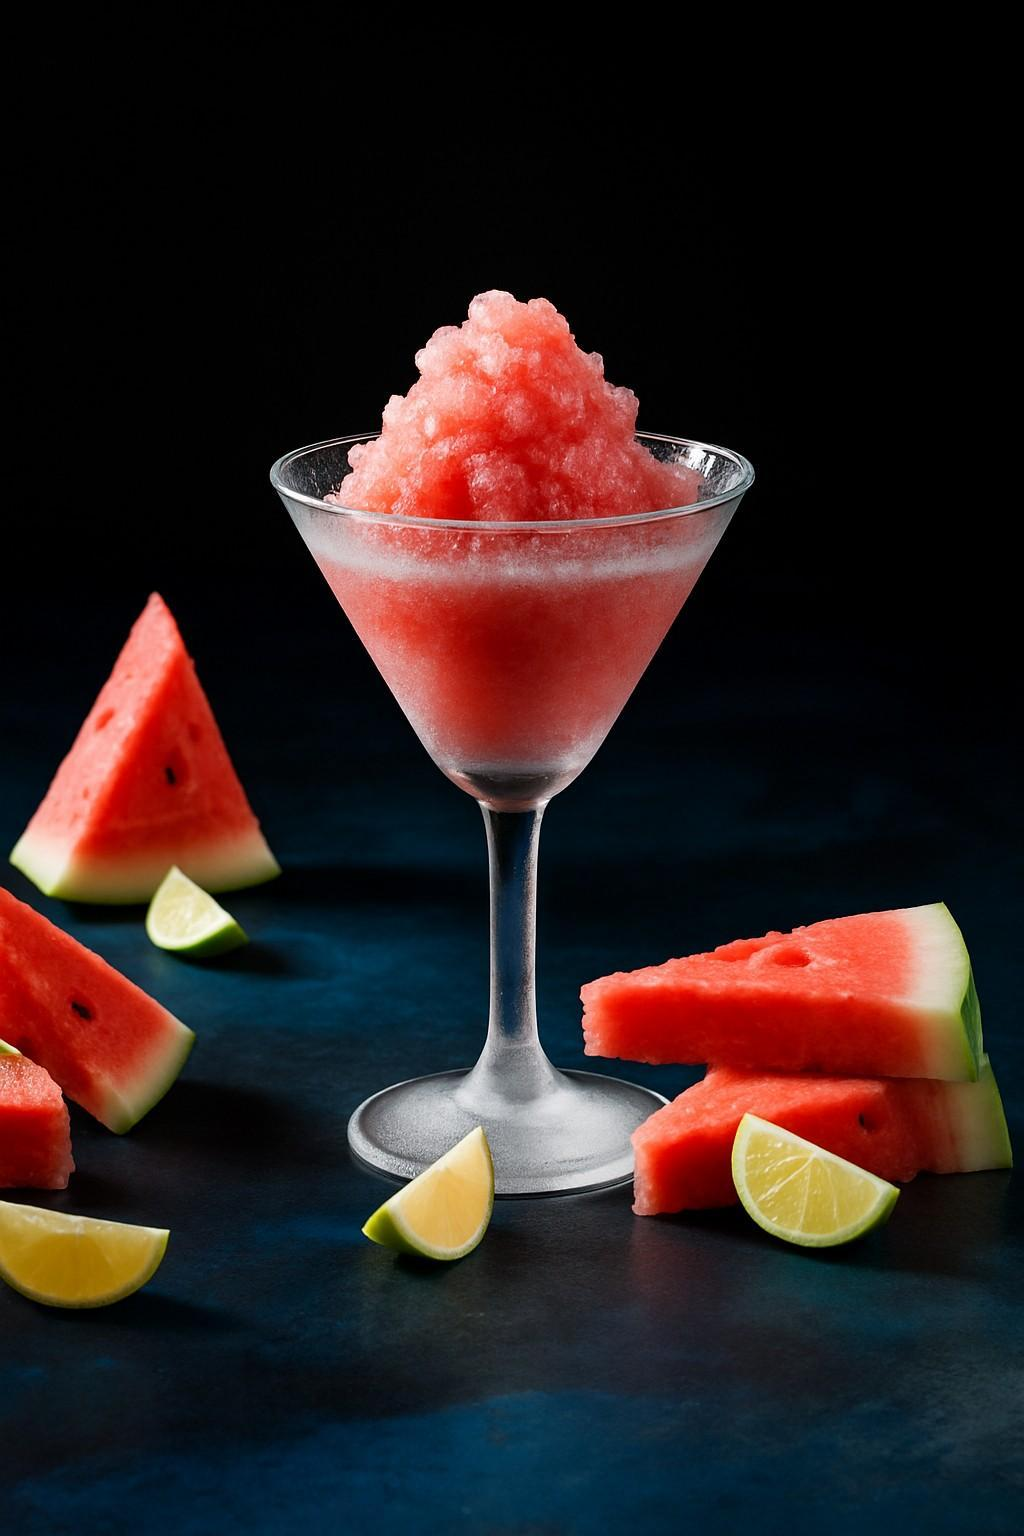}}
\end{minipage}
\hfill
\begin{minipage}[t]{0.19\linewidth}
\centering
\adjustbox{width=\linewidth,height=\minipageheightakIntermediate,keepaspectratio}{\includegraphics{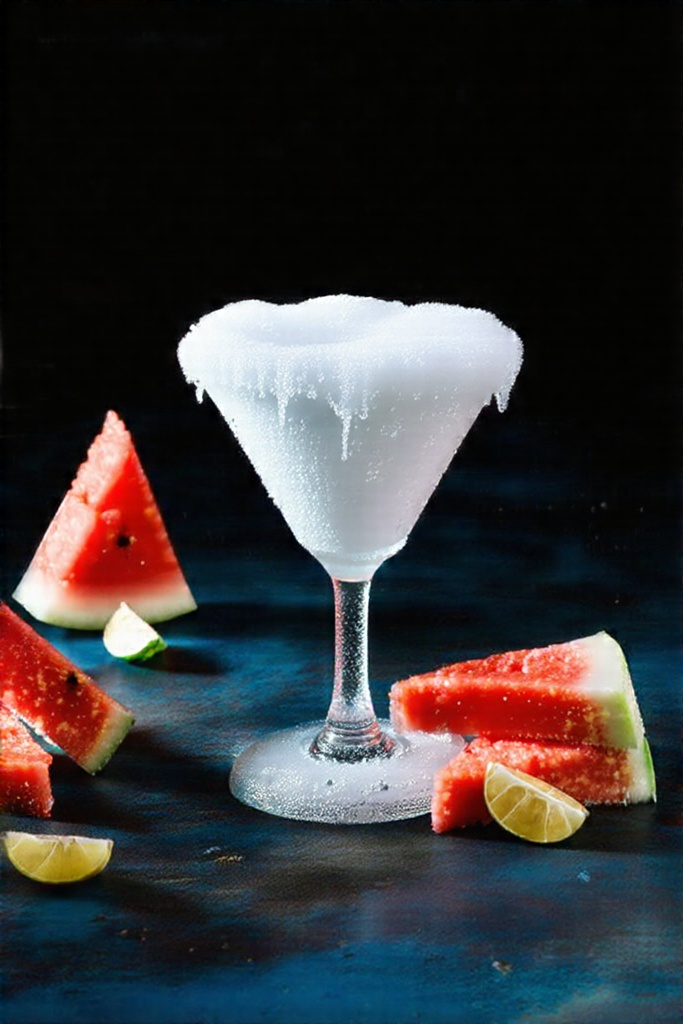}}
\end{minipage}
\hfill
\begin{minipage}[t]{0.19\linewidth}
\centering
\adjustbox{width=\linewidth,height=\minipageheightakIntermediate,keepaspectratio}{\includegraphics{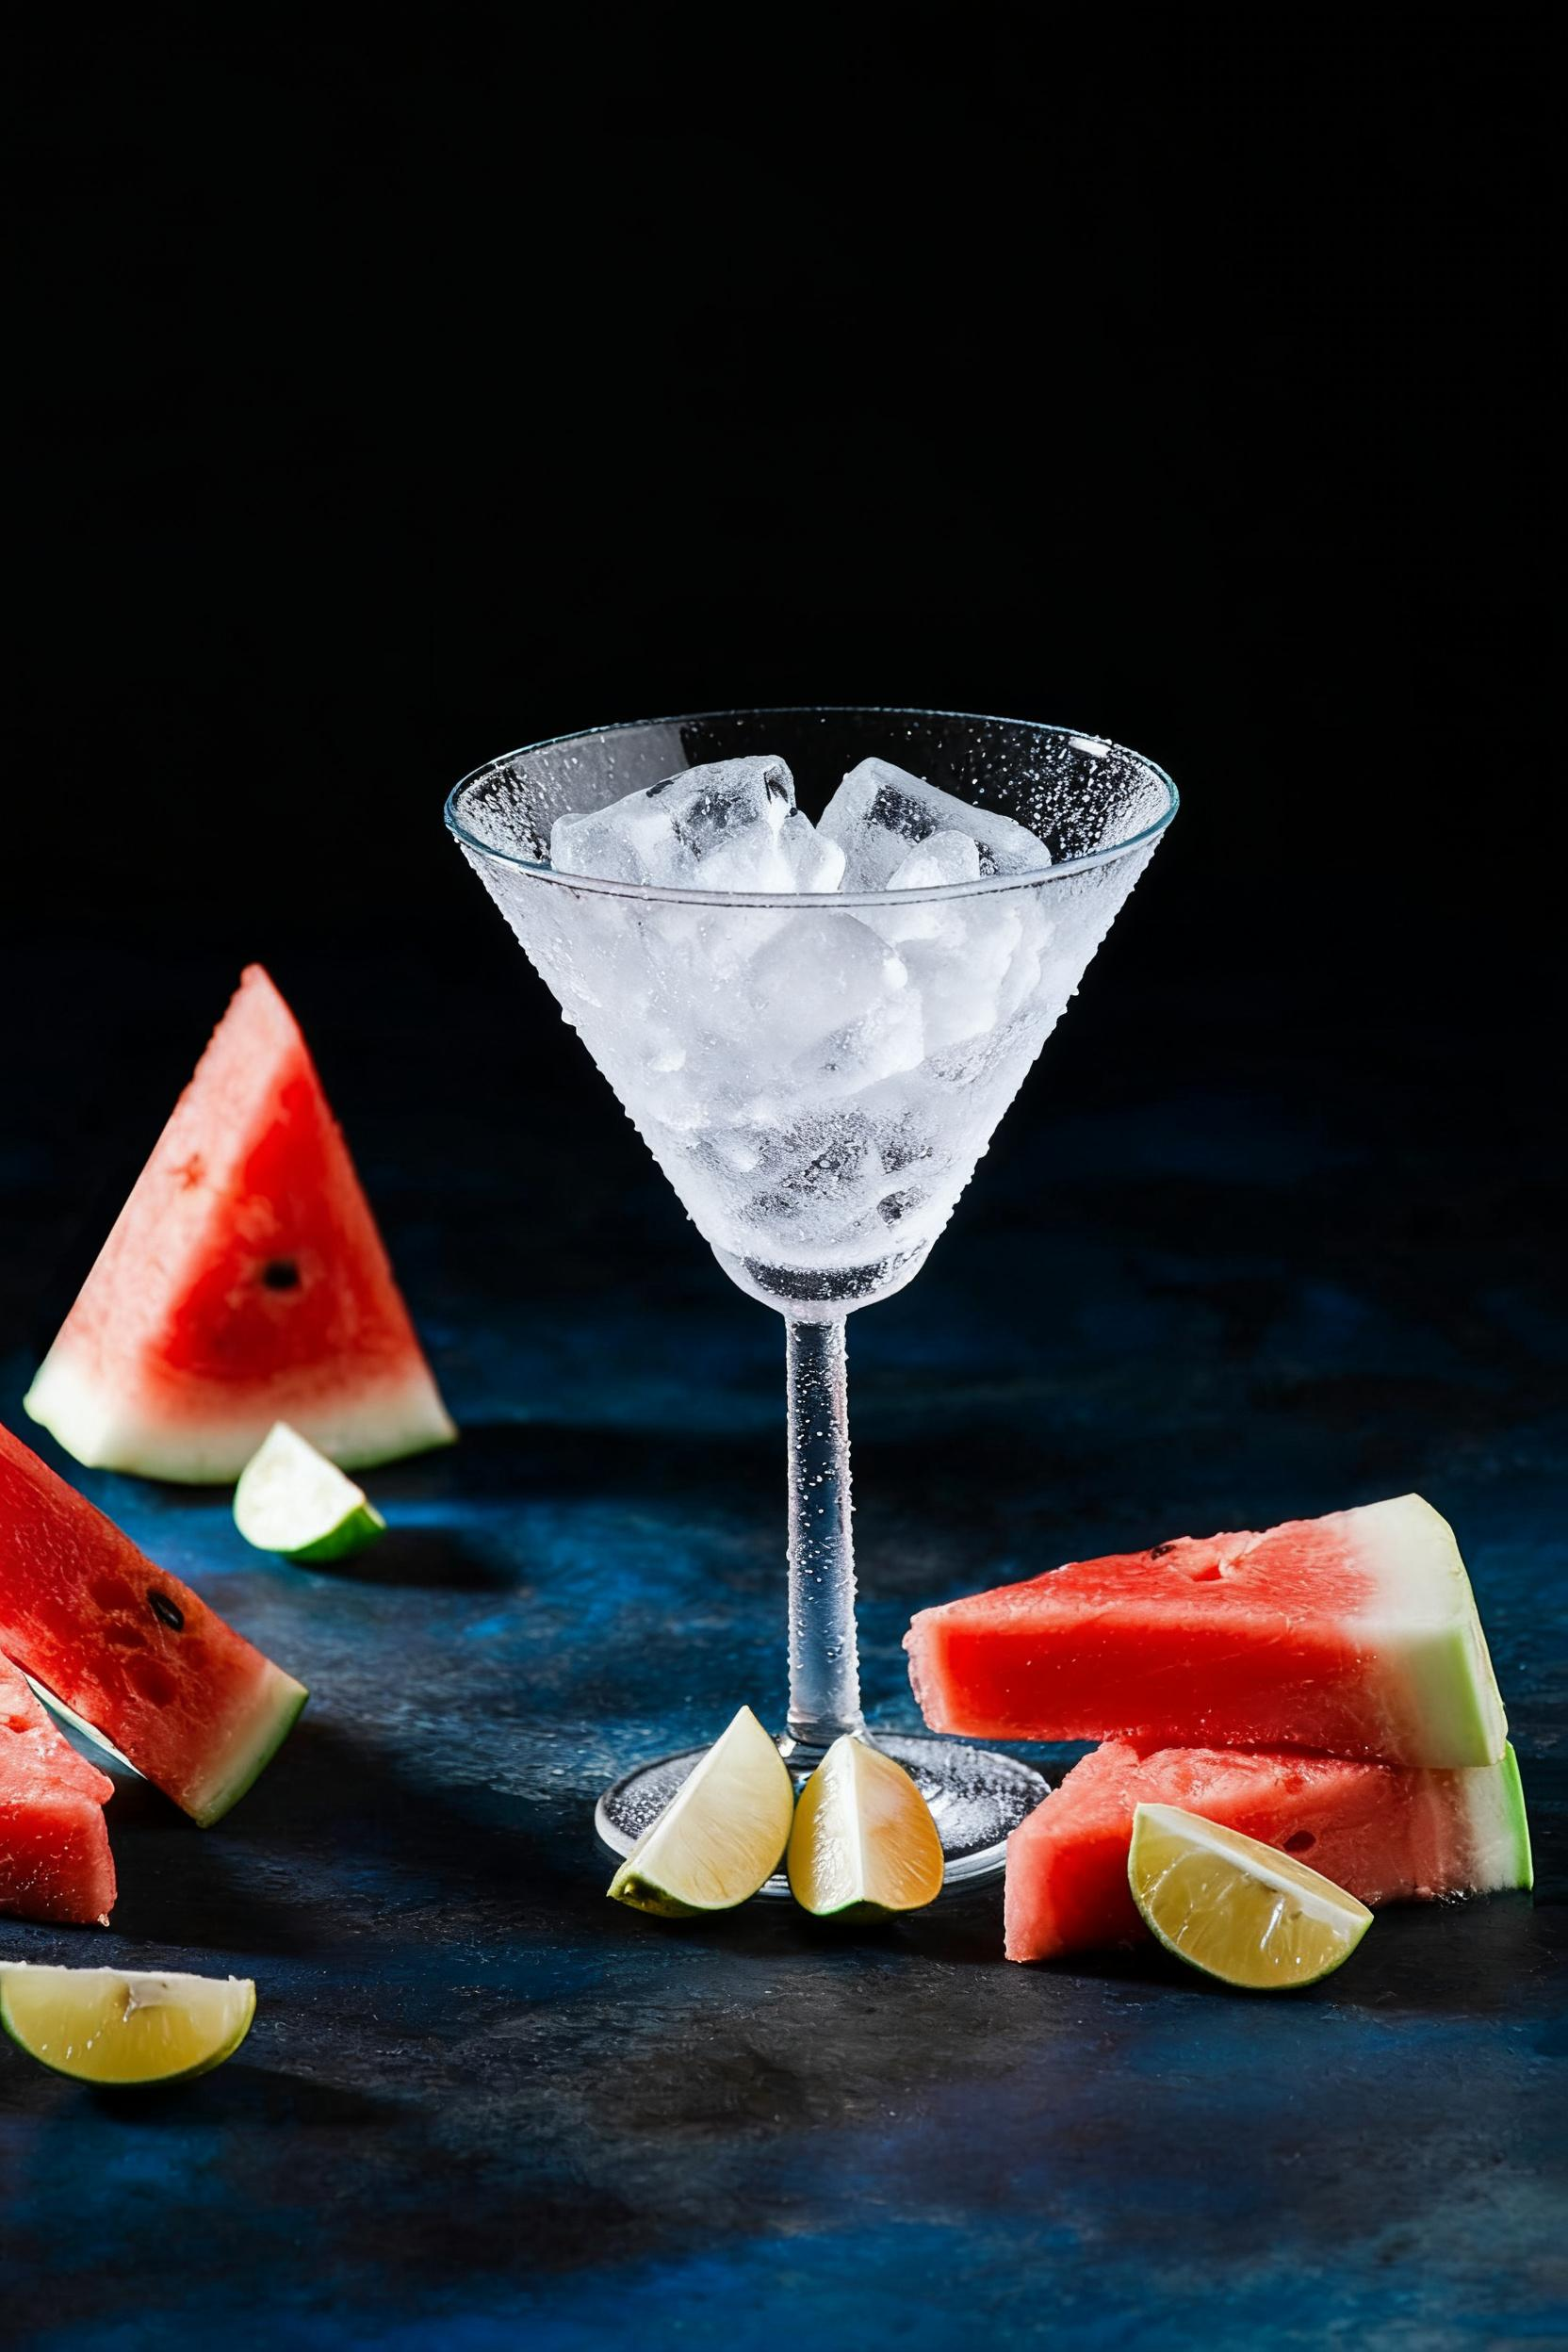}}
\end{minipage}
\hfill
\begin{minipage}[t]{0.19\linewidth}
\centering
\adjustbox{width=\linewidth,height=\minipageheightakIntermediate,keepaspectratio}{\includegraphics{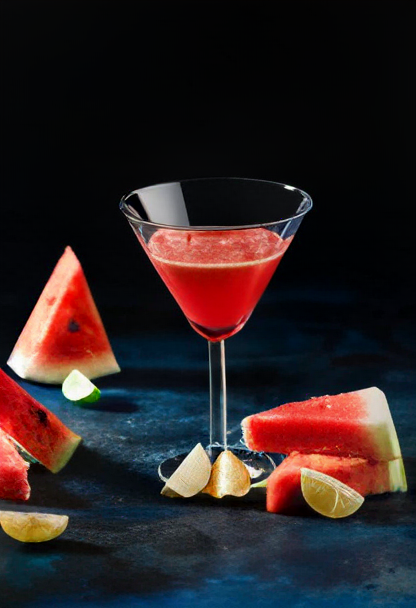}}
\end{minipage}
\hfill
\begin{minipage}[t]{0.19\linewidth}
\centering
\adjustbox{width=\linewidth,height=\minipageheightakIntermediate,keepaspectratio}{\includegraphics{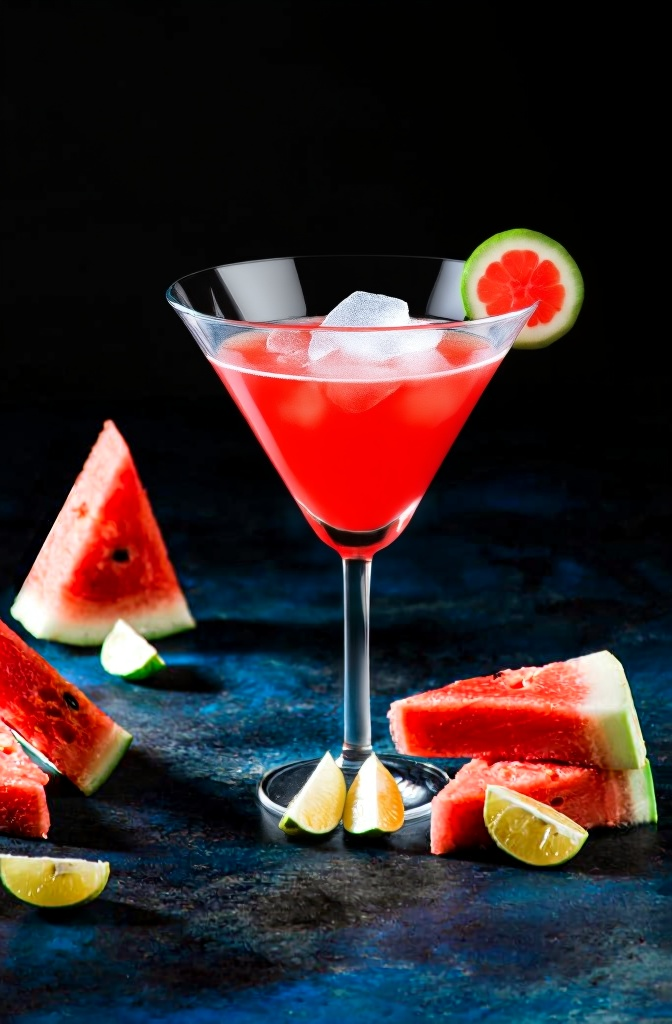}}
\end{minipage}\\
\begin{minipage}[t]{0.19\linewidth}
\centering
\vspace{-0.7em}\textbf{\footnotesize GPT-Image 1}    
\end{minipage}
\hfill
\begin{minipage}[t]{0.19\linewidth}
\centering
\vspace{-0.7em}\textbf{\footnotesize HiDream-E1.1}    
\end{minipage}
\hfill
\begin{minipage}[t]{0.19\linewidth}
\centering
\vspace{-0.7em}\textbf{\footnotesize Seedream 4.0}    
\end{minipage}
\hfill
\begin{minipage}[t]{0.19\linewidth}
\centering
\vspace{-0.7em}\textbf{\footnotesize DiMOO}    
\end{minipage}
\hfill
\begin{minipage}[t]{0.19\linewidth}
\centering
\vspace{-0.7em}\textbf{\footnotesize OmniGen2}    
\end{minipage}\\

\end{minipage}

\vspace{2em}

\begin{minipage}[t]{\linewidth}
\textbf{Explicit Prompt:} Transform the ivy leaves in the photo into a fully dry state. Remove every surface water droplet and any wet ... \\
\vspace{-0.5em}
\end{minipage}
\begin{minipage}[t]{\linewidth}
\centering
\newsavebox{\tmpboxalExplicit}
\newlength{\minipageheightalExplicit}
\sbox{\tmpboxalExplicit}{
\begin{minipage}[t]{0.19\linewidth}
\centering
\includegraphics[width=\linewidth]{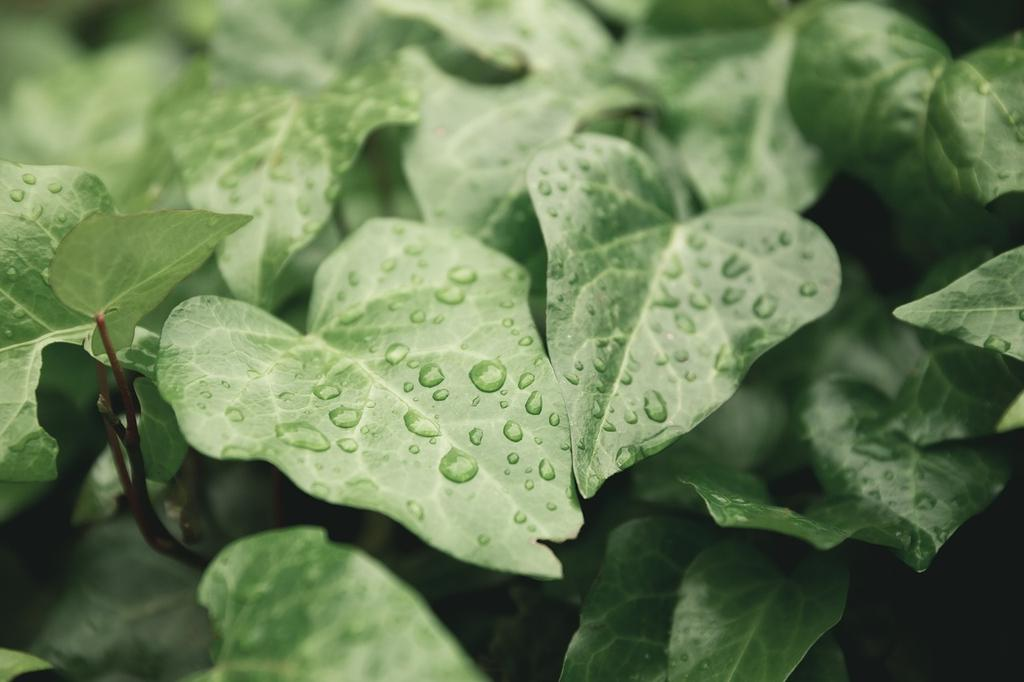}
\vspace{-1em}\textbf{\footnotesize Input}
\end{minipage}
}
\setlength{\minipageheightalExplicit}{\ht\tmpboxalExplicit}
\begin{minipage}[t]{0.19\linewidth}
\centering
\adjustbox{width=\linewidth,height=\minipageheightalExplicit,keepaspectratio}{\includegraphics{iclr2026/figs/final_selection/State__Local__explicit_0406_nature-4485461_1280_State_Local_dry/input.png}}
\end{minipage}
\hfill
\begin{minipage}[t]{0.19\linewidth}
\centering
\adjustbox{width=\linewidth,height=\minipageheightalExplicit,keepaspectratio}{\includegraphics{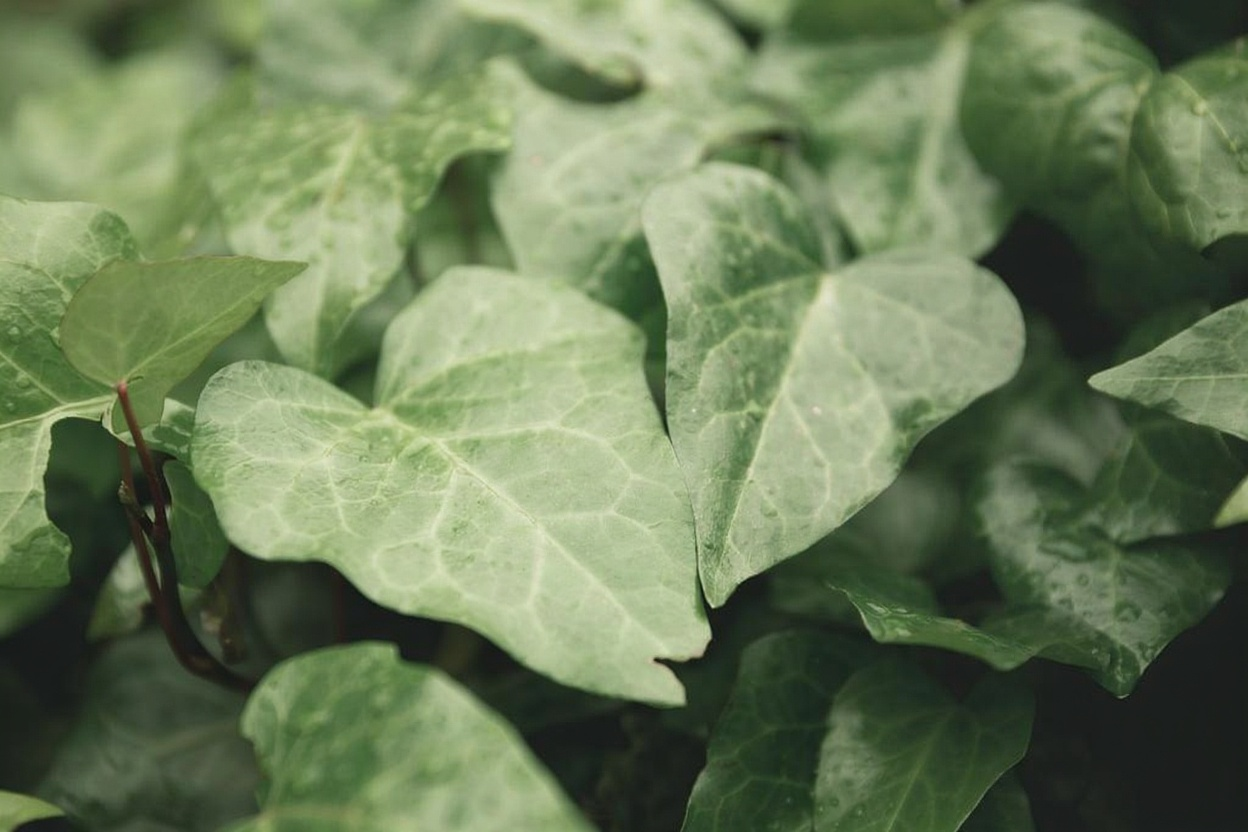}}
\end{minipage}
\hfill
\begin{minipage}[t]{0.19\linewidth}
\centering
\adjustbox{width=\linewidth,height=\minipageheightalExplicit,keepaspectratio}{\includegraphics{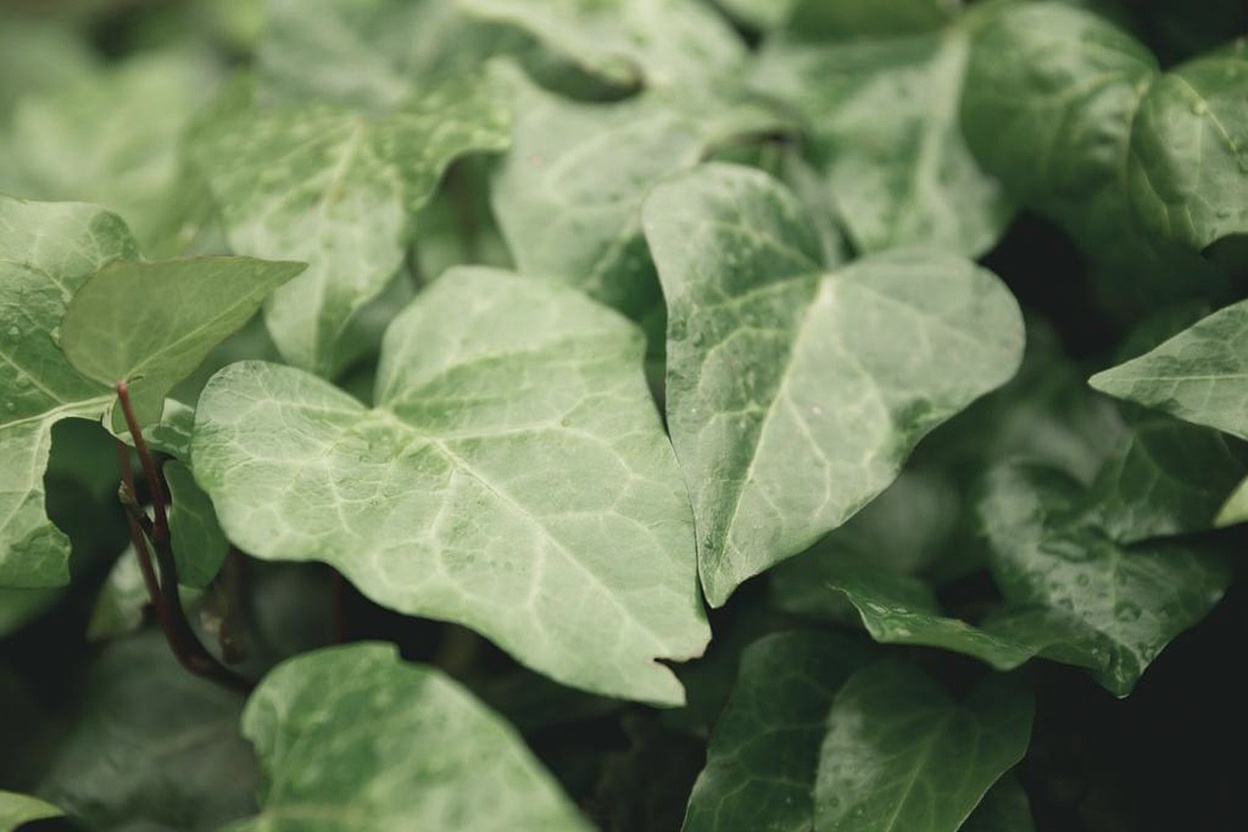}}
\end{minipage}
\hfill
\begin{minipage}[t]{0.19\linewidth}
\centering
\adjustbox{width=\linewidth,height=\minipageheightalExplicit,keepaspectratio}{\includegraphics{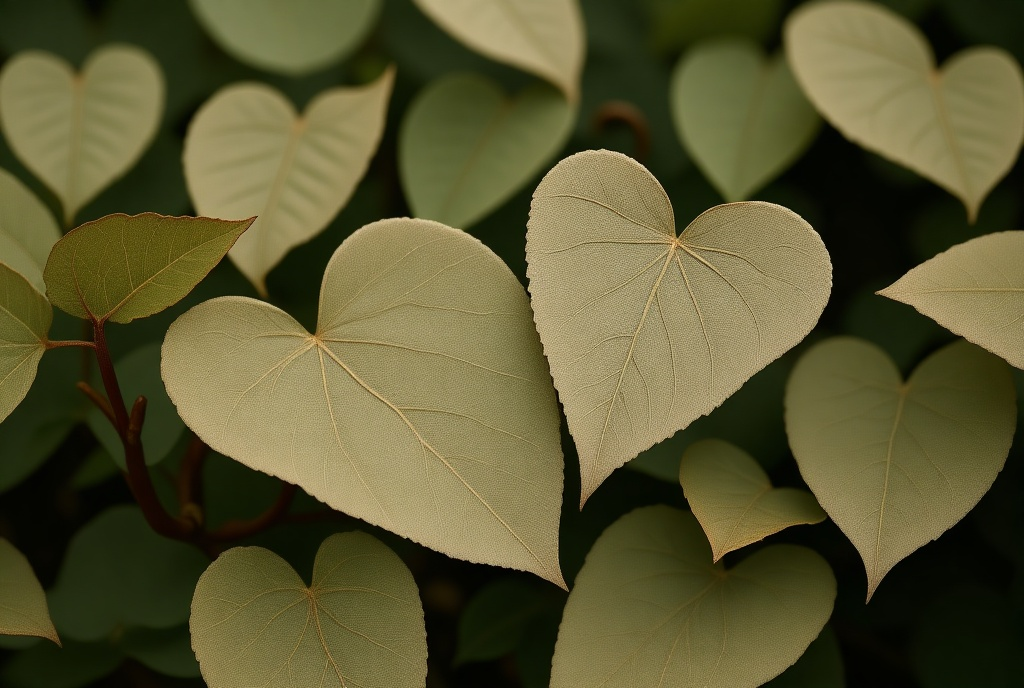}}
\end{minipage}
\hfill
\begin{minipage}[t]{0.19\linewidth}
\centering
\adjustbox{width=\linewidth,height=\minipageheightalExplicit,keepaspectratio}{\includegraphics{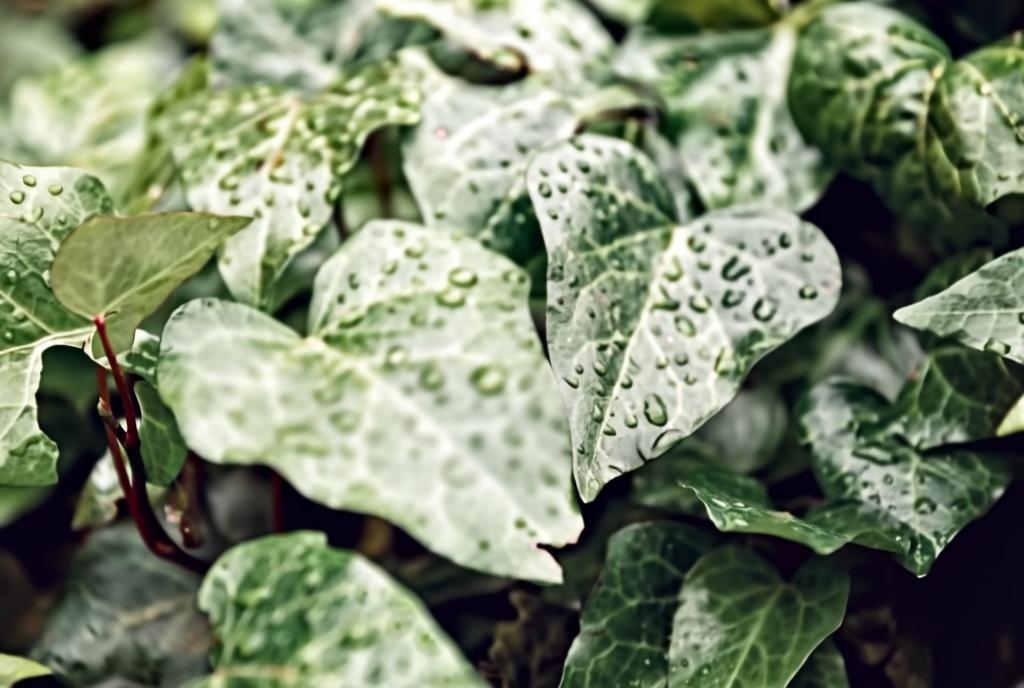}}
\end{minipage}\\
\begin{minipage}[t]{0.19\linewidth}
\centering
\vspace{-0.7em}\textbf{\footnotesize Input}    
\end{minipage}
\hfill
\begin{minipage}[t]{0.19\linewidth}
\centering
\vspace{-0.7em}\textbf{\footnotesize Ours}    
\end{minipage}
\hfill
\begin{minipage}[t]{0.19\linewidth}
\centering
\vspace{-0.7em}\textbf{\footnotesize Flux.1 Kontext}    
\end{minipage}
\hfill
\begin{minipage}[t]{0.19\linewidth}
\centering
\vspace{-0.7em}\textbf{\footnotesize BAGEL}    
\end{minipage}
\hfill
\begin{minipage}[t]{0.19\linewidth}
\centering
\vspace{-0.7em}\textbf{\footnotesize BAGEL-Think}    
\end{minipage}\\
\begin{minipage}[t]{0.19\linewidth}
\centering
\adjustbox{width=\linewidth,height=\minipageheightalExplicit,keepaspectratio}{\includegraphics{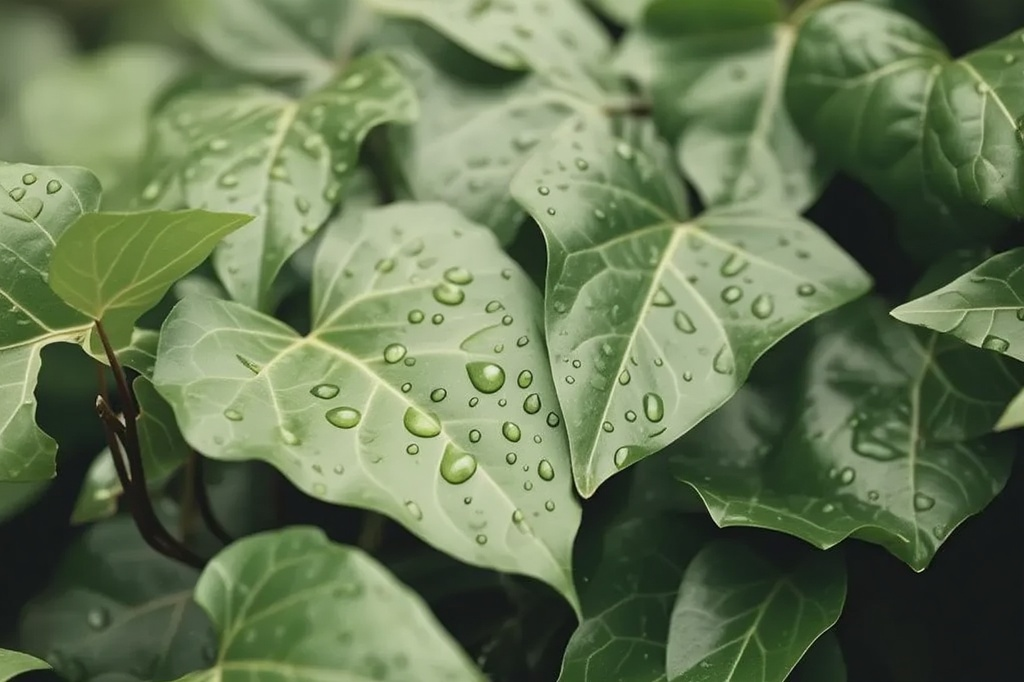}}
\end{minipage}
\hfill
\begin{minipage}[t]{0.19\linewidth}
\centering
\adjustbox{width=\linewidth,height=\minipageheightalExplicit,keepaspectratio}{\includegraphics{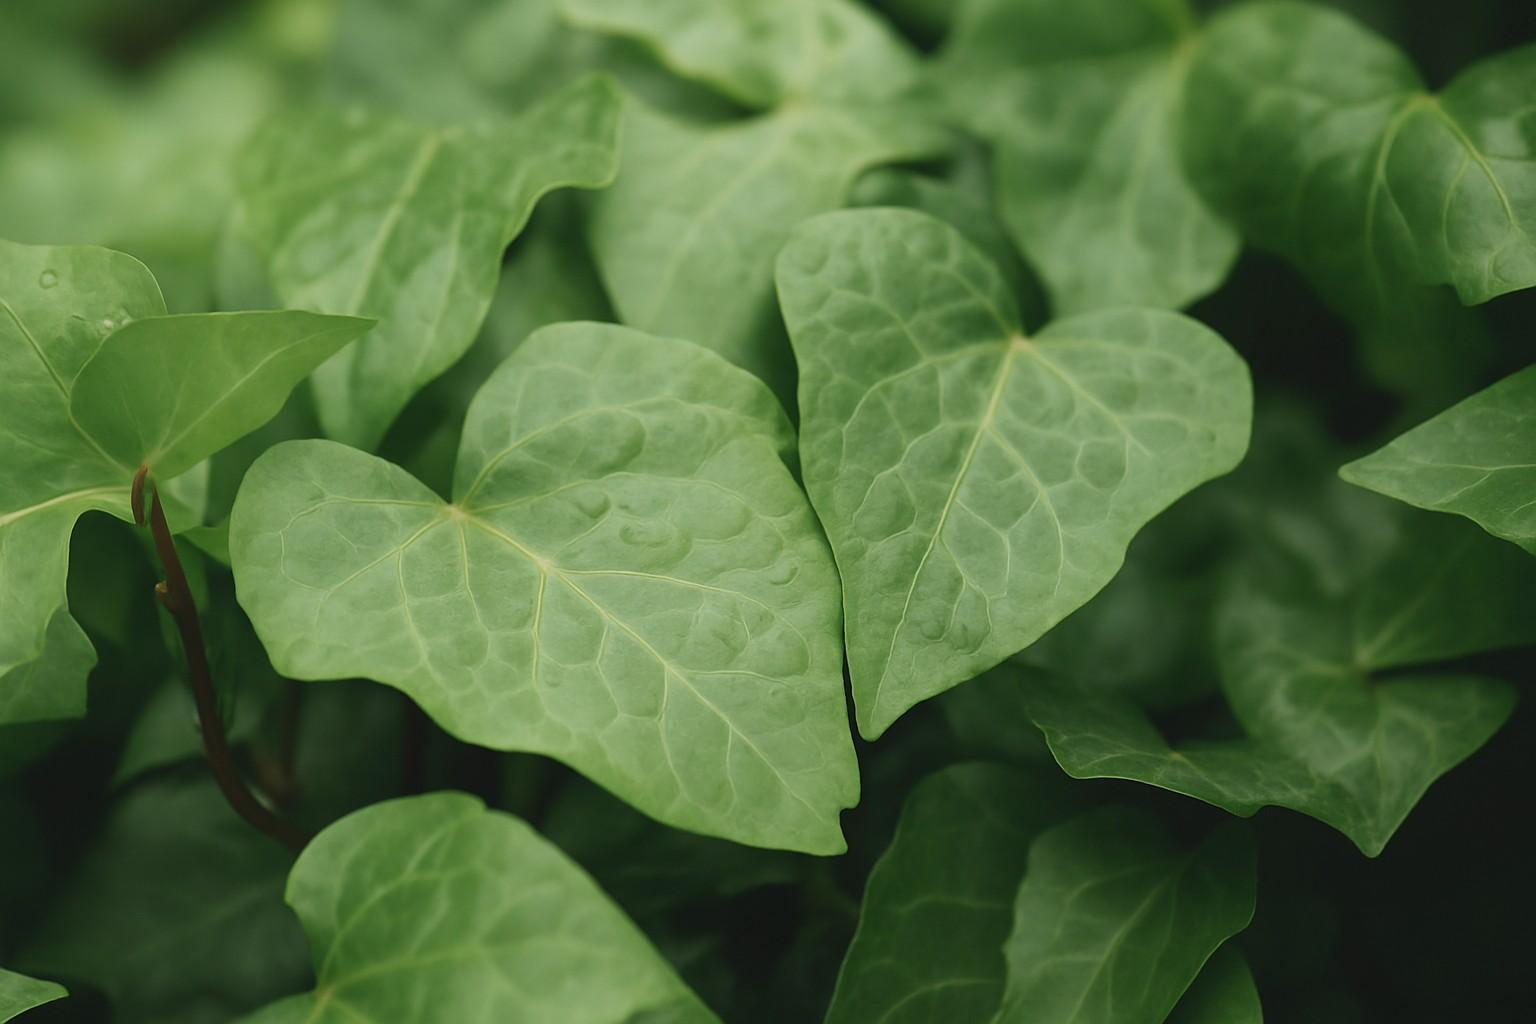}}
\end{minipage}
\hfill
\begin{minipage}[t]{0.19\linewidth}
\centering
\adjustbox{width=\linewidth,height=\minipageheightalExplicit,keepaspectratio}{\includegraphics{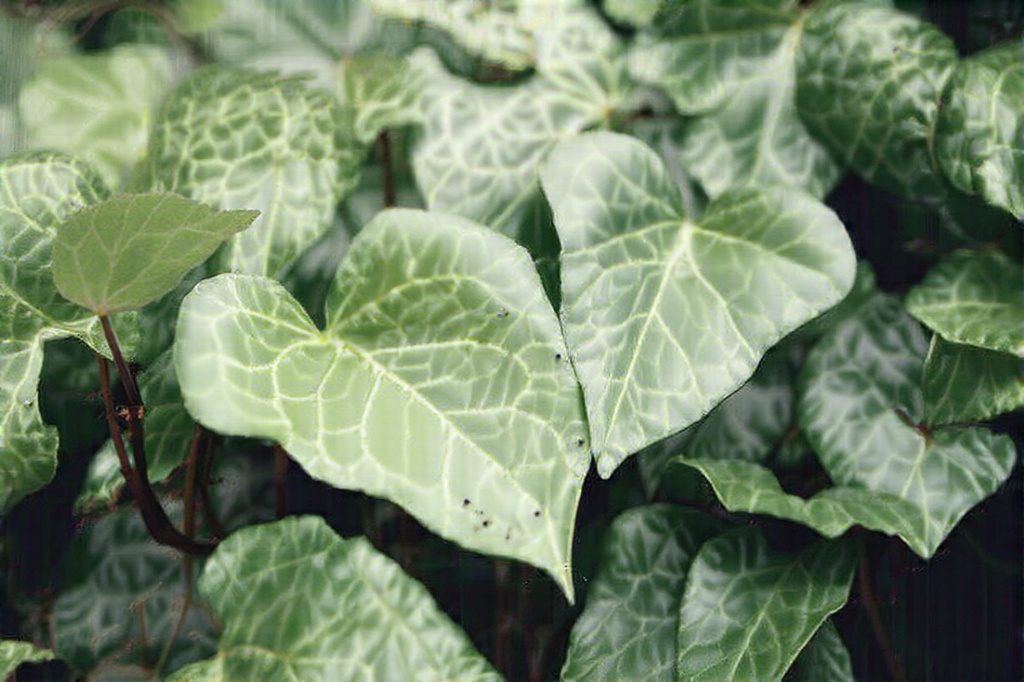}}
\end{minipage}
\hfill
\begin{minipage}[t]{0.19\linewidth}
\centering
\adjustbox{width=\linewidth,height=\minipageheightalExplicit,keepaspectratio}{\includegraphics{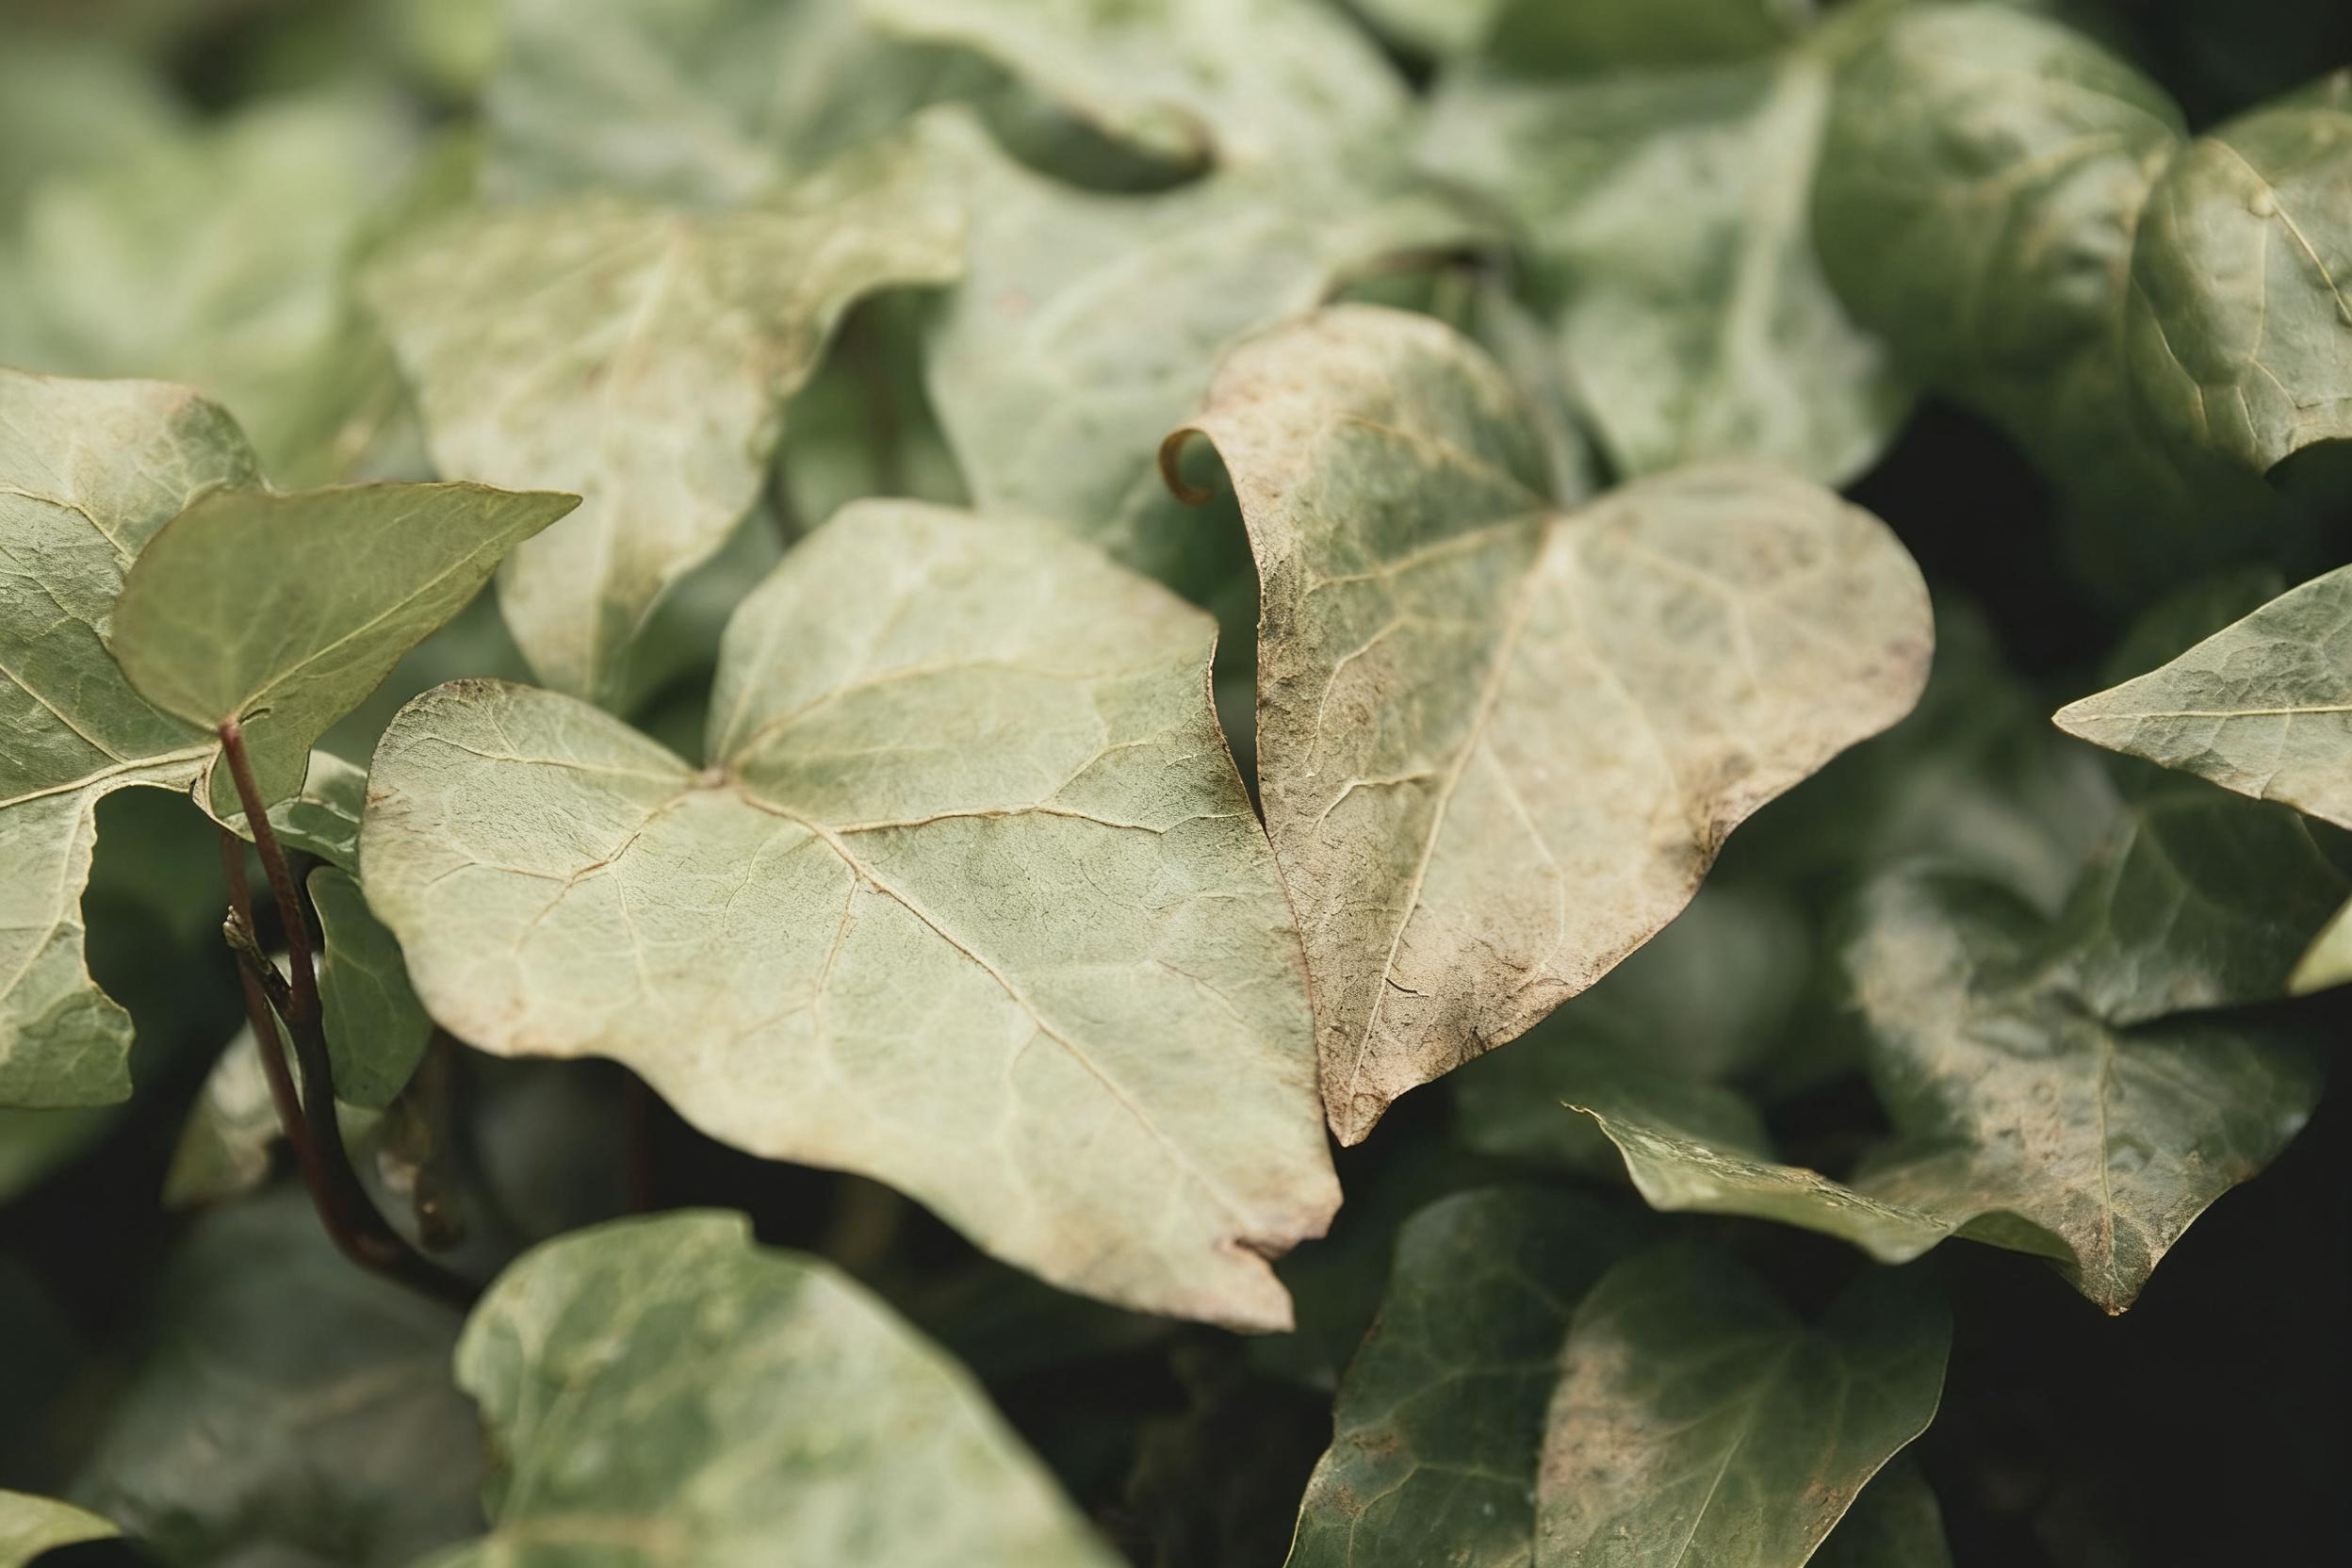}}
\end{minipage}
\hfill
\begin{minipage}[t]{0.19\linewidth}
\centering
\adjustbox{width=\linewidth,height=\minipageheightalExplicit,keepaspectratio}{\includegraphics{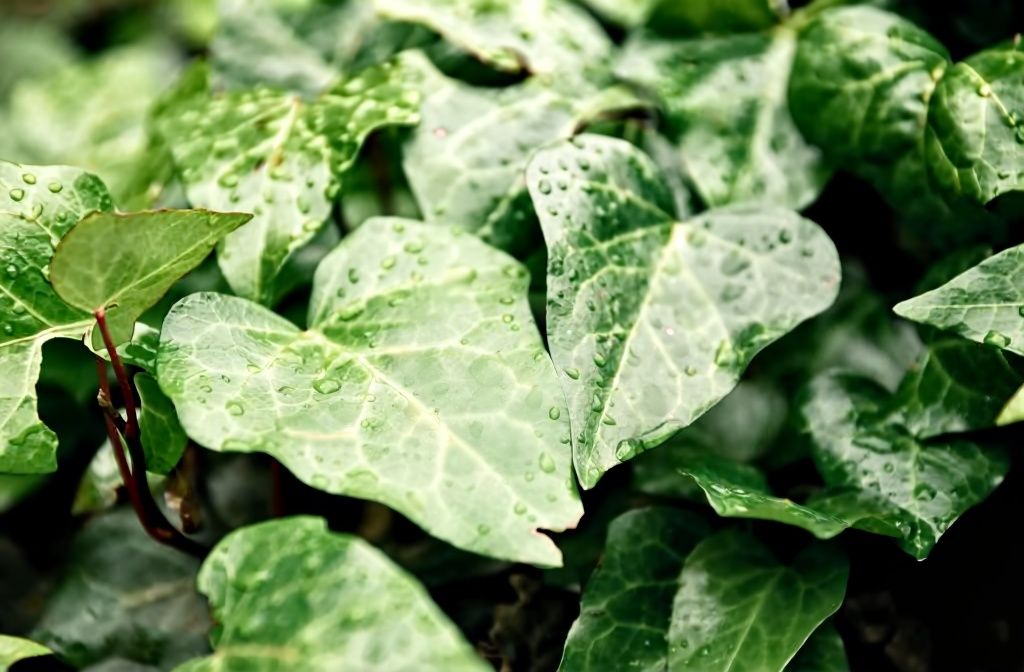}}
\end{minipage}\\
\begin{minipage}[t]{0.19\linewidth}
\centering
\vspace{-0.7em}\textbf{\footnotesize Step1X-Edit}    
\end{minipage}
\hfill
\begin{minipage}[t]{0.19\linewidth}
\centering
\vspace{-0.7em}\textbf{\footnotesize GPT-Image 1}    
\end{minipage}
\hfill
\begin{minipage}[t]{0.19\linewidth}
\centering
\vspace{-0.7em}\textbf{\footnotesize HiDream-E1.1}    
\end{minipage}
\hfill
\begin{minipage}[t]{0.19\linewidth}
\centering
\vspace{-0.7em}\textbf{\footnotesize Seedream 4.0}    
\end{minipage}
\hfill
\begin{minipage}[t]{0.19\linewidth}
\centering
\vspace{-0.7em}\textbf{\footnotesize OmniGen2}    
\end{minipage}\\

\end{minipage}

\caption{Examples of how models follow the law of local in state transition (intermediate \& explicit propmts).}
\label{supp:fig:local_state transition_Explicit}
\end{figure}
